# Supplementary material for: Reinforcement Learning under Latent Dynamics: Toward Statistical and Algorithmic Modularity
Source: arXiv:2410.17904 source file (2024-10-23)
Supplement: Supplementary file 1 [file appendix_reductions.tex]

\pacomment{TODO: this needs to go somewhere else}

\pacomment{Introducing the concept of reductions}

\subsection{Reductions via Latent Algorithms}\label{sec:latent}

\pacomment{move this earlier -- make it more general}

We consider a \Replearn procedure which chooses a set of features based on observational data and a latent algorithm \Alglat which chooses policies based on the newly chosen features. \Alglat takes as input a dataset over $\cS \times \cA \times [0,1] \times \cS$ tuples and outputs a policy as well as a prediction. Formally, we consider the following interaction protocol:

\begin{algoshort}[Reduction]\label{alg:reduction}\,
\begin{enumerate}
	\item Let $\cD^t = \{(x^i_h, a^i_h, r^i_h, x^i_{h+1})\}_{i=1:(t-1), h=1:H}$ be the dataset of all the trajectories up until time $t$.
	\item Based on $\cD^t$, \Replearn will choose a set of features $\Phi_t$. 
	\item For each $\phi \in \Phi_t$, we call \Alglat on the dataset 
\[
	 \cD^t_{\phi} \coloneqq \{(\phi(x^i_h), a^i_h, r^i_h, \phi(x^i_{h+1}))\}_{i=1:(t-1), h=1:H}.
\]
	\Alglat with $\cD^t_\phi$ outputs a policy $\pi^t_{\phi} \in \Pilat$ and a prediction $f^t_{\phi} \in \bbF_\lat$.
	\item \textbf{Online case:} We run \textsc{tournament} on the pairs $\{(\pi^t_\phi,f^t_\phi)\}_{\phi \in \Phi_t}$ to select $\phi_t$ (without deploying any $\pi^t_\phi$).
	\item We deploy the policy $\pi^t_\obs \coloneqq \pi^t_{\phi_t} \circ \phi_t \in \Piobs$. 
\end{enumerate}
\end{algoshort}

\subsection{Confounded POMDPs}\label{sec:confounded-pomdps}

At time $t$ we have a dataset $\cD^t_\phi$ collected from $\pi^1_\obs, \cdots, \pi^{t-1}_\obs$. From the point of view of \Alglat, this data is generated from a POMDP with \textit{confounded} policies $\pi^1_\obs \cdots \pi^{t-1}_\obs$. Formally the POMDP is defined by
\begin{definition}[$\phi$-based POMDP]
The POMDP $\wtM_{\phi}$ generated by $\Mstarobs$ and $\phi$ is defined by:
\begin{enumerate}
	\item \underline{Latent} state space $\cX$
	\item Action space $\cA$
	\item \underline{Observation} state space $\cS$
	\item Latent reward functions $\Rstarobsh: \cX \times \cA \rightarrow [0,1]$
	\item Latent dynamics $\Pstarobsh: \cX \times \cA \rightarrow \Delta(\cX)$
	\item (Deterministic) observation distribution $\cO: \cX \rightarrow \cS$ defined by $\cO(x) = \phi(x)$, 
	\item Horizon $H$
	\item Initial latent distribution $\Pstarobs(x_0 \mid \emptyset)$
\end{enumerate}	
\end{definition}

Note that the latent space \textit{for the POMDP} is the observation space of the rich observation MDP $\Mstar$, and vice-versa. \pacomment{find some terminology to distinguish this}

As a graphical model, the primitives which define all joint distributions $\wtM^{\piobs}_\phi(x_I,s_J,a_K)$ for any subset $I,J,K \subseteq [H]$ are:
\begin{enumerate}
	\item $\bbP(x_0) = \Pstar_{\obs,0}(x_0 \mid \emptyset)$
	\item $\bbP(s_h \mid x_h) = \delta_{\phi(x_h)}(s_h)$
	\item $\bbP(x_{h+1} \mid x_h,a_h) = \Pstarobsh(x_{h+1} \mid x_h,a_h)$
	\item and $\bbP(a_h \mid x_h) = \piobs(a_h \mid x_h)$
\end{enumerate}  

For example, we have
\begin{align*}
	\wtP^{\piobs}_\phi(s_{h+1} \mid s_{1:h},a_{1:h}) &= \frac{1}{\wtP^{\piobs}_\phi(s_{1:h},a_{1:h})}\wtP^{\piobs}_\phi(s_{h+1},s_{1:h},a_{1:h}) \\
	&= \frac{1}{\wtP^{\piobs}_\phi(s_{1:h},a_{1:h})}\sum_{x_{1:h+1}} \wtP^{\piobs}_\phi(s_{h+1},s_{1:h},a_{1:h},x_{1:h+1})\\
	&= \frac{1}{\wtP^{\piobs}_\phi(s_{1:h},a_{1:h})}\sum_{x_{1:h+1}} \bbP(x_1)\left( \prod_{i \leq h} \bbP(s_i \mid x_i) \piobs(a_i \mid x_i) \bbP(x_{i+1} \mid x_i,a_i)\right) \bbP(s_{h+1} \mid x_{h+1}) 
\end{align*}

Similarly, the primitives which define all joint distributions $\wtM^{\pilat}_\phi(x_I,s_J,a_K)$ for any subset $I,J,K \subseteq [H]$ are
\begin{enumerate}
	\item $\bbP(x_0) = \Pstar_{\obs,0}(x_0 \mid \emptyset)$
	\item $\bbP(s_h \mid x_h) = \delta_{\phi(x_h)}(s_h)$
	\item $\bbP(x_{h+1} \mid x_h,a_h) = \Pstarobsh(x_{h+1} \mid x_h,a_h)$
	\item and $\bbP(a_h \mid s_h) = \pilat(a_h \mid s_h)$,
\end{enumerate}  
which is just the regular (unconfounded) POMDP dynamics with latent policies.

We write $\wtE^\pi_{\phi} \coloneqq \En^{\wtM_\phi,\pi}$ for expectations over the latent space $\cS \times \cA$ according to $\wtM_{\phi}$. Due to confounding, we can write $\wtE^{\piobs}_\phi$.

Note that due to confounding, $\wtP^{\piobs}_{\phi}(s_{h+1} = \cdot \mid s_1, a_1, \dots, s_h, a_h) \neq \wtP_{\phi}(s_{h+1} = \cdot \mid s_1, a_1, \dots, s_h, a_h)$. However, we do have that $\wtP^{\pilat}_{\phi}(s_{h+1} = \cdot \mid s_1, a_1, \dots, s_h, a_h) = \wtP_{\phi}(s_{h+1} = \cdot \mid s_1, a_1, \dots, s_h, a_h)$
